# Supplementary material for: MVControl: Adding Conditional Control to Multi-view Diffusion for Controllable Text-to-3D Generation
Source: arXiv:2311.14494 source file (2023-11-27)
Supplement: Supplementary file 1 [file supp_method.tex]

% General
We first review relevant methods, including MVDream \cite{shi2023mvdream}, ControlNet \cite{zhang2023controlnet} and SDS \cite{poole2022dreamfusion} in Section \ref{subsec:preliminary}. Then, we analyze the strategy of introducing additional spatial conditioning to MVDream by training a multi-view ControlNet in Section \ref{subsec:MVControl}. Finally in Section \ref{subsec:3dgen}, based on the trained multi-view ControlNet, we propose the realization of controllable 3D content generation using SDS loss with hybrid diffusion priors as guidance.

% Neural representation of sharp scene
\subsection{Preliminary}
\label{subsec:preliminary}

\PAR{Diffusion models} predict the score function $\nabla_{\mathbf{x}}\log p_{data}(\mathbf{x})$ in the data space under different noise level $t\sim \mathcal{U}(0, T)$, so as to guide the sampling process denoising from pure noise $x_T\sim \mathcal{N}(\mathbf{0}, \mathbf{I})$ to clean data $x_0$. To learn the denoising score, noises of different scale are added to $x_0$ with pre-defined schedule $\alpha_t\in(0,1)$ and $\bar{\alpha}_t:=\prod_{s=1}^{t}\alpha_{s}$, according to:
\begin{equation}
	x_t=\sqrt{\bar{\alpha}_t}x_0 + \sqrt{1-\bar{\alpha}_t}\epsilon, \text{where } \epsilon \sim \mathcal{N}(\mathbf{0}, \mathbf{I}) \label{eq:1}
\end{equation}
then the diffusion model parameterized by $\phi$ is trained by minimizing the noise reconstruction loss:
\begin{equation}
	\mathcal{L}_{\textrm{diffusion}}=\mathbb{E}_{t,\epsilon}\lbrack\Vert \epsilon_{\phi}(x_t, t)-\epsilon \Vert _2 ^2\rbrack. \label{eq:2}
\end{equation}
Once the model is trained, it can be iteratively applied to denoise a pure noise to sample a clean data. The readers can refer to \cite{ho2020denoising, song2020score} for more detailed illustration about diffusion models.

\PAR{MVDream} \cite{shi2023mvdream} is a multi-view diffusion model fine-tuned based on the large-scale pre-trained image diffusion model, Stable-Diffusion (SD) \cite{rombach2022stablediffusion}. While SD generates one image for one sampling process, MVDream generates 4 images, $\mathcal{X}=\{x^{(k)}; x^{(k)} \in \mathbb{R}^{H\times W\times C}\}_{k=1}^4$, of one object's 4 consistent views $\mathcal{V}=\{v^{(k)}; v^{(k)} \in \mathbb{R}^{4\times 4}\}_{k=1}^4$ that are 90 degrees apart from each other and at the same elevation. To ensure the interaction of features among different views, MVDream replaces self attention layers of SD to cross-view attentions, which concatenate the patches of all views before attention computation. And they further utilize a small MLP (Multi-layer Perceptron) $\mathcal{M}_{\text{camera}}$ that projects the camera matrices into embeddings $e_{v^{(k)}}=\mathcal{M}_{\text{camera}}(\text{flatten}(v^{(k)}))$, which are injected to whole model by adding them to timestep embeddings $e_t$, so as to make the prediction view-conditioned.

\PAR{ControlNet} \cite{zhang2023controlnet} is trained as a plug-in module of SD. It introduces another spatial condition aside from text prompt to SD by taking the spatial conditioning image (canny edges, sketches, depth maps, \etc.) as input. ControlNet is initialized by directly copying the structure and weights of SD's encoder blocks and mid block, and adding some zero-ly initialized 1x1 convolutions as connections between it and SD. With those connections, the feature map output by each inner layer of ControlNet is injected to its corresponding symmetric layer in SD's UNet decoder, so as to control the sampling process of SD.

\PAR{Score Distillation Sampling} (SDS) \cite{poole2022dreamfusion, lin2023magic3d} enables leveraging the priors of pre-trained text-to-image diffusion models to facilitate text-conditioned generation in other domains, particularly 3D content generation by distilling the 2D image priors from the diffusion models into differentiable 3D representations, \eg, NeRF. Specifically, given a pre-trained diffusion model $\epsilon_{\phi}$, SDS optimizes a set of parameters $\theta$ of a differentiable parametric image generator or renderer $g$, using the gradient of the loss $\mathcal{L}_{SDS}$ with respect to $\theta$:
\begin{equation}
	\nabla_{\theta}\mathcal{L}_{\textrm{SDS}}(\phi, \mathbf{x})=\mathbb{E}_{t,\epsilon}\lbrack w(t)(\hat{\epsilon}_\phi-\epsilon)\frac{\partial{z_t}}{\partial{\theta}}\rbrack, \label{eq:3}
\end{equation}
where $\mathbf{x}=g(\theta, c)$ is an image rendered by $\theta$ under a camera pose $c$, $w(t)$ is a weighting function depending on the timestep $t$ and $z_t$ is the noisy image input to diffusion model by adding Gaussian noise $\epsilon$ to $\mathbf{x}$ corresponding to the $t$-th timestep according to Eq. \ref{eq:1}. In practice, the values of timestep $t$ and Gaussian noise $\epsilon$ are randomly sampled at every optimization step. 

\subsection{Multi-view ControlNet}
\label{subsec:MVControl}

While ControlNet has provided a successful strategy to adding additional conditioning to the pre-trained SD, which is to train another neural network module to inject features into the frozen SD, and thanks to the recently released multi-view diffusion prior, MVDream, it's natural to train a multi-view version of ControlNet to control the forward process of MVDream. 
What's more, since MVDream doesn't change the architecture of original SD and ControlNet also inherits the structure of SD, it remarks us to follow this idea that is to preserve the backbone of the base model as much as possible to maximize the retention of base model's prior knowledge, which is, developing our model based on a pre-trained 2D ControlNet.

Firstly, we conduct an experiment to evaluate the performance of pre-trained 2D ControlNet checkpoints when attaching them with MVDream. The experiment results are shown in Figure \ref{fig:1}, where we can see that the pre-trained 2D ControlNet checkpoint still can control the generation process of MVDream even when MVDream is on full-conditioned (when cross-attention and camera matrix embeddings are enabled). We also tried to set the first of four generated views as indentity view and only apply ControlNet's feature on the identity view, in order to see whether the cross-view attention can broadcast the control signals from identity view to the other views. The result shows that ...

Although the control signal from ControlNet is not consistent for multi-view generation, it can serve as a good start point to develop our model since it can already provide a precise conditioning signal corresponding to the input spatial conditioning image to MVDream. 
Our experiments also show that directly training from a 2D ControlNet checkpoint converges much faster than initializing from MVDream's weights, and the relevant results can be found in our [supplementary materials].
The framework of our proposed method is shown as Figure \ref{fig:network}, where the whole MVDream is frozen and we only train the MVControl part. To make the control signals from the ControlNet part view-dependent, following MVDream, we replace all the self attention layers with cross-view attentions, where all patches of input feature maps of different views are concatenated together before QKA calculation and reshape back afterwards. 

Another keypoint is the way to introduce view (camera matrix) conditions: whether relative or absolute camera pose should we use? Setting the view of given conditioning image as reference view, We find it hard to converge if the generated target views don't contain reference view. Since the 2D ControlNet checkpoint has owned the capacity to reconstruction the image of reference view, it will be much easier to learn multi-view control signals with the reference view image as the pivot. Hence, our solution can be formulated as controlling MVDream to generate 4 images $\mathcal{X}=\{x^{(k)}; x^{(k)}\in \mathbb{R}^{H\times W\times C}\}_{k=1}^{4}$ belonging to 4 orthogonal views $\mathcal{V}^*=\{v_*^{(k)}\}_{k=1}^{4}$ with one of them as the reference view $v_r$, defined by the given conditioning image $c\in\mathbb{R}^{H\times W\times C}$, \eg, $v_*^{(1)}=v_r$. In this way, since we can't get access to the correct absolute camera poses of the reference view so as to the 4 target views, we can only use camera poses relative to the reference view which is set to a identity pose in the world coordinate system. By setting the identity pose as position at $(r, 0, 0)$ and looking at the world center, the positions of $\mathcal{V}^*$ can be all determined, where $r$ is the camera distance to world center.  

But directly utilizing the embeddings of relative camera matrices is conflict with absolute camera pose conditioned MVDream and will introduce additional error to the whole system. 
What's more, if inheriting the setting in 2D ControlNet that the conditioning image is embedded by a block $\mathcal{E}_c$, that consists of several successive convolution layers, to the same shape as noisy images to add to them, multi-view consistency can't be ensured since the conditioning embedding is all the same for different views. 

To overcome these issues, we present a new simple but effective embedding mechanism. As shown in Figure \ref{fig:network-b}, let's denote the feature map of the conditioning image in $\mathcal{E}_c$ before the last convolution out layer as $\Psi$, to make the condition image embedding view- and time-dependent, we add a new shallow MLP $\mathcal{M}_1$ to project the original view-conditioned timestep embedding $e_{t, v_*^{(k)}}=e_t+e_{{v_*}^{(k)}}$ to a proper shape and add it to $\Psi$, \eg, $\Psi_{t, v_*^{(k)}}=\Psi+\mathcal{M}_1(e_{t, v_*^{(k)}})$. 
What's more, we further add an embedding head $\mathcal{M}_2$ paralleled with the final convolution out layer to predict a new embedding $e^g_{c, t, v_*^{(k)}}=\mathcal{M}_2(\Psi_{t, v_*^{(k)}})$ to globally control the forward process of both MVControl and MVDream part by replacing $e_{v_*}^{(k)}$ and adding it to the timestep embeddings at every inner layers. And the outputs of last convolution layer, $e^l_{c, t, v_*^{(k)}}$, can work as local control signals by adding to the noisy image of different views.

\subsection{Controllable 3D Content Generation}
\label{subsec:3dgen}
Upon MVControl is trained, it can be utilized for controllable 3D content generation through SDS optimization pipeline.
In this part, we adopt a hybrid diffusion prior consisting of Stable-Diffusion and our MVControl, whose parameters are $\psi$ and $\phi$ respectively, to guide a coarse-to-fine optimization process, where we first optimize a coarse neural surface \cite{wang2021neus}, and then in the fine texture optimization stage, the coarse geometry is transformed to a deformable mesh \cite{shen2021dmtet} for optimizing realistic and coherent texture with geometry fixed. As for the hybrid diffusion prior, the MVControl part works as a strong consistent geometry guidance under 4 canonical views of the 3D object, and Stable-Diffusion part provides fine geometry and texture sculpting at the other randomly sampled views.
In the following part, we denote the 4 canonical views together as $\mathcal{V}_*$ and the images rendered under those views as $\mathcal{X}_*\in\mathbb{R}^{4\times H\times W\times C}$.

\subsubsection{Coarse Geometry Stage}
At this stage, we aim to generate a 3D model whose geometry is consistent with the input condition image. 
While our MVControl can already provide consistent geometry constrains from 4 fixed canonical views, it's still not enough to recover a plausible geometry from the sparse 4 views. Hence, we propose to incorporating another 2D diffusion model, stable-diffusion, to provide a semantic guidance under those views other than the 4 canonical view and so as to sculpt the geometry meeting the distribution described by the condition image.

Specifically, supposings a differentiable renderer $g(\cdot)$ the parameters of 3D representation as $\theta$, we render the images $\mathcal{X}_*=g(\theta, \mathcal{V}_*)$ under 4 canonical views and image $x_r=g(\theta, v_r)$ under a randomly sampled view $v_r$. 
Then the the gradient of hybrid SDS loss can be computed as:

\begin{equation}
	\nabla_\theta\mathcal{L}_{SDS}^{hybrid}=\lambda_1 \nabla_\theta\mathcal{L}_{SDS}^{SD} + \lambda_2 \nabla_\theta\mathcal{L}_{SDS}^{MV},
\end{equation}

where $\nabla_\theta\mathcal{L}_{SDS}^{SD}$ is the SDS gradient distillated from Stable-Diffusion taking $x_r$ as input and $\nabla_\theta\mathcal{L}_{SDS}^{MV}$ is that distillated from our MVControl with $\mathcal{X}_*$ and $\mathcal{V}_*$ as input. $\lambda_1$ and $\lambda_2$ are the weight of them two respectively. 
Considering the fixed 4 views are participated in every optimization step, while the other views are randomly sampled, we give $\lambda_2$ a small value and $\lambda_1$ a large one to balance the weights of views.

While classifier-free guidance (CFG) \cite{ho2022cfg} has become a necessary technique when doing diffusion sampling, we should consider the CFG scale for each of our diffusion priors. 
To order to enforce the optimization process align to the distribution defined by our MVControl, we apply a large CFG scale $s_{MV}^g=50$ for $\nabla_\theta\mathcal{L}_{SDS}^{MV}$. 
And due to the gap between the generation domain of Stable-Diffusion (2D) and MVControl (3D), we choose to use a relatively small CFG scale $s_{SD}^g=10$ for $\nabla_\theta\mathcal{L}_{SDS}^{SD}$ in avoid of the against of its guidance with that of MVControl and so as to impede optimization process.
Here, following \cite{shi2023mvdream}, we compute $\nabla_\theta\mathcal{L}_{SDS}^{MV}$ through $x_0$-reconstruction formulation to alleviate the color saturation from large CFG scale by applying CFG rescale trick \cite{lin2023common}:
\begin{equation}
	\nabla_\theta\mathcal{L}_{SDS}^{MV}(\psi, \mathcal{X}_*, \mathcal{V}_*)=\mathbb{E}_{t, \epsilon}\lbrack \Vert \mathcal{X}_*-\hat{\mathcal{X}}_0 \Vert _2^2 \rbrack.
\end{equation}
Here $\hat{\mathcal{X}}_0$ is the estimated clean images of the 4 noisy input from $\epsilon_\psi(z_t(\mathcal{X}_*);y, t, \mathcal{V}_*)$ and its gradient is detached. And as for the computation of $\nabla_\theta\mathcal{L}_{SDS}^{SD}$, we refer to the normal SDS calculation defined in Eq. \ref{eq:3} since it uses a small CFG scale.
For regularization, we use the eikonal loss proposed by \cite{wang2021neus} to constrain the SDF values to a more plausible form. 

\subsubsection{Fine Texture Stage}
In fine stage, we extract the previously obtained coarse neural surface to DMTet \cite{shen2021dmtet} and then only optimize its texture with geometry fixed.
